# Supplementary material for: Quantification of electron correlation effects - Quantum Information Theory versus Method of Increments
Source: arXiv:1808.10200 ancillary file (2018-12-11)
Supplement: Supplementary file 1 [file SI.pdf]

#MO 1

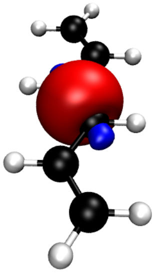

$\epsilon_i = -0.8598\ E_\mathrm{h}$
$\varepsilon_i = -0.0002\ E_\mathrm{h}$
$S_i = 0.0109$
$|-\rangle = 0.000$
$|\downarrow\rangle = 0.001$
$|\uparrow\rangle = 0.001$
$|\downarrow\uparrow\rangle = 0.999$

#MO 2

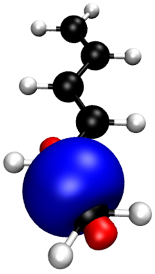

$\epsilon_i = -0.8582\ E_\mathrm{h}$
$\varepsilon_i = -0.0003\ E_\mathrm{h}$
$S_i = 0.0126$
$|-\rangle = 0.000$
$|\downarrow\rangle = 0.001$
$|\uparrow\rangle = 0.001$
$|\downarrow\uparrow\rangle = 0.999$

#MO 3

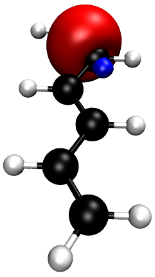

$\epsilon_i = -0.8582\ E_\mathrm{h}$
$\varepsilon_i = -0.0003\ E_\mathrm{h}$
$S_i = 0.0127$
$|-\rangle = 0.000$
$|\downarrow\rangle = 0.001$
$|\uparrow\rangle = 0.001$
$|\downarrow\uparrow\rangle = 0.998$

#MO 4

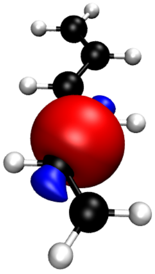

$\epsilon_i = -0.8077\ E_\mathrm{h}$
$\varepsilon_i = -0.0006\ E_\mathrm{h}$
$S_i = 0.0174$
$|-\rangle = 0.000$
$|\downarrow\rangle = 0.001$
$|\uparrow\rangle = 0.001$
$|\downarrow\uparrow\rangle = 0.998$

#MO 5

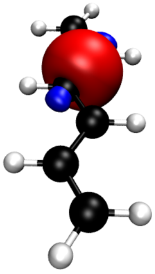

$\epsilon_i = -0.8077\ E_\mathrm{h}$
$\varepsilon_i = -0.0006\ E_\mathrm{h}$
$S_i = 0.0175$
$|-\rangle = 0.000$
$|\downarrow\rangle = 0.001$
$|\uparrow\rangle = 0.001$
$|\downarrow\uparrow\rangle = 0.998$

#MO 6

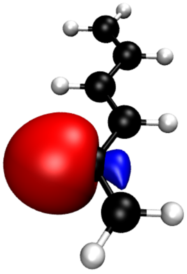

$\epsilon_i = -0.7076\ E_\mathrm{h}$
$\varepsilon_i = -0.0014\ E_\mathrm{h}$
$S_i = 0.0252$
$|-\rangle = 0.001$
$|\downarrow\rangle = 0.001$
$|\uparrow\rangle = 0.001$
$|\downarrow\uparrow\rangle = 0.997$

#MO 7

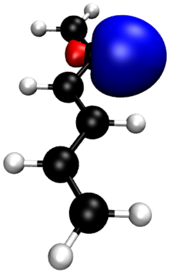

$\epsilon_i = -0.7076\ E_\mathrm{h}$
$\varepsilon_i = -0.0014\ E_\mathrm{h}$
$S_i = 0.0253$
$|-\rangle = 0.001$
$|\downarrow\rangle = 0.001$
$|\uparrow\rangle = 0.001$
$|\downarrow\uparrow\rangle = 0.997$

#MO 8

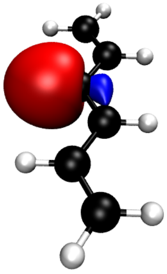

$\epsilon_i = -0.7070\ E_\mathrm{h}$
$\varepsilon_i = -0.0015\ E_\mathrm{h}$
$S_i = 0.0289$
$|-\rangle = 0.001$
$|\downarrow\rangle = 0.001$
$|\uparrow\rangle = 0.001$
$|\downarrow\uparrow\rangle = 0.996$

FIG. S1. Polyacetelene: Pipek-Mezey localized active space molecular orbitals #1 to #8 with their corresponding diagonal Fock matrix element $\epsilon_i$, 1-orbital increment $\varepsilon_i$, 1-orbital entropy $S_i$ and orbital occupations $\omega_{i,\alpha} = \{|-\rangle, |\downarrow\rangle, |\uparrow\rangle, |\downarrow\uparrow\rangle\}$. Isosurfaces are plotted at $|\psi(\vec{r})| = 0.05\ a_0^{-1.5}$).

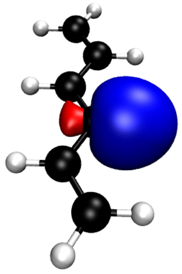

#MO 9

$\epsilon_i = -0.7070\ E_\mathrm{h}$
$\varepsilon_i = -0.0015\ E_\mathrm{h}$
$S_i = 0.0288$
$|-\rangle = 0.001$
$|\downarrow\rangle = 0.001$
$|\uparrow\rangle = 0.001$
$|\downarrow\uparrow\rangle = 0.996$

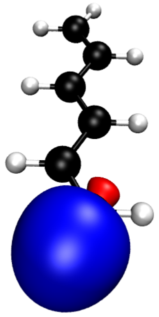

#MO 10

$\epsilon_i = -0.7011\ E_\mathrm{h}$
$\varepsilon_i = -0.0013\ E_\mathrm{h}$
$S_i = 0.0234$
$|-\rangle = 0.001$
$|\downarrow\rangle = 0.001$
$|\uparrow\rangle = 0.001$
$|\downarrow\uparrow\rangle = 0.997$

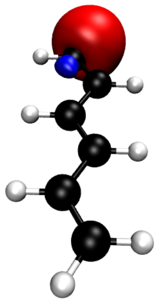

#MO 11

$\epsilon_i = -0.7011\ E_\mathrm{h}$
$\varepsilon_i = -0.0013\ E_\mathrm{h}$
$S_i = 0.0234$
$|-\rangle = 0.001$
$|\downarrow\rangle = 0.001$
$|\uparrow\rangle = 0.001$
$|\downarrow\uparrow\rangle = 0.997$

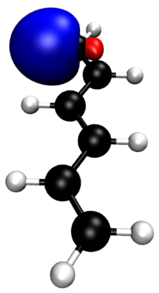

#MO 12

$\epsilon_i = -0.7003\ E_\mathrm{h}$
$\varepsilon_i = -0.0014\ E_\mathrm{h}$
$S_i = 0.0251$
$|-\rangle = 0.001$
$|\downarrow\rangle = 0.001$
$|\uparrow\rangle = 0.001$
$|\downarrow\uparrow\rangle = 0.997$

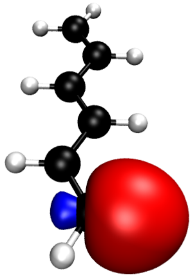

#MO 13

$\epsilon_i = -0.7003\ E_\mathrm{h}$
$\varepsilon_i = -0.0014\ E_\mathrm{h}$
$S_i = 0.0251$
$|-\rangle = 0.001$
$|\downarrow\rangle = 0.001$
$|\uparrow\rangle = 0.001$
$|\downarrow\uparrow\rangle = 0.997$

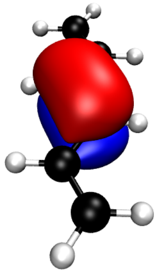

#MO 14

$\epsilon_i = -0.3891\ E_\mathrm{h}$
$\varepsilon_i = -0.0129\ E_\mathrm{h}$
$S_i = 0.2006$
$|-\rangle = 0.020$
$|\downarrow\rangle = 0.009$
$|\uparrow\rangle = 0.009$
$|\downarrow\uparrow\rangle = 0.962$

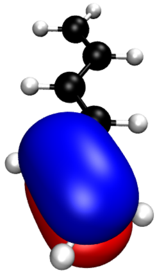

#MO 15

$\epsilon_i = -0.3769\ E_\mathrm{h}$
$\varepsilon_i = -0.0137\ E_\mathrm{h}$
$S_i = 0.1787$
$|-\rangle = 0.022$
$|\downarrow\rangle = 0.006$
$|\uparrow\rangle = 0.006$
$|\downarrow\uparrow\rangle = 0.966$

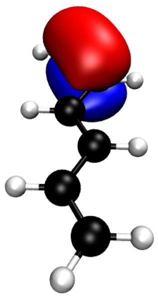

#MO 16

$\epsilon_i = -0.3769\ E_\mathrm{h}$
$\varepsilon_i = -0.0137\ E_\mathrm{h}$
$S_i = 0.1796$
$|-\rangle = 0.022$
$|\downarrow\rangle = 0.006$
$|\uparrow\rangle = 0.006$
$|\downarrow\uparrow\rangle = 0.966$

FIG. S2. Polyacetelene: Pipek-Mezey localized active space molecular orbitals #9 to #16 with their corresponding diagonal Fock matrix element $\epsilon_i$, 1-orbital increment $\varepsilon_i$, 1-orbital entropy $S_i$ and orbital occupations $\omega_{i,\alpha} = \{|-\rangle, |\downarrow\rangle, |\uparrow\rangle, |\downarrow\uparrow\rangle\}$. Isosurfaces are plotted at $|\psi(\vec{r})| = 0.05\ a_0^{-1.5}$).

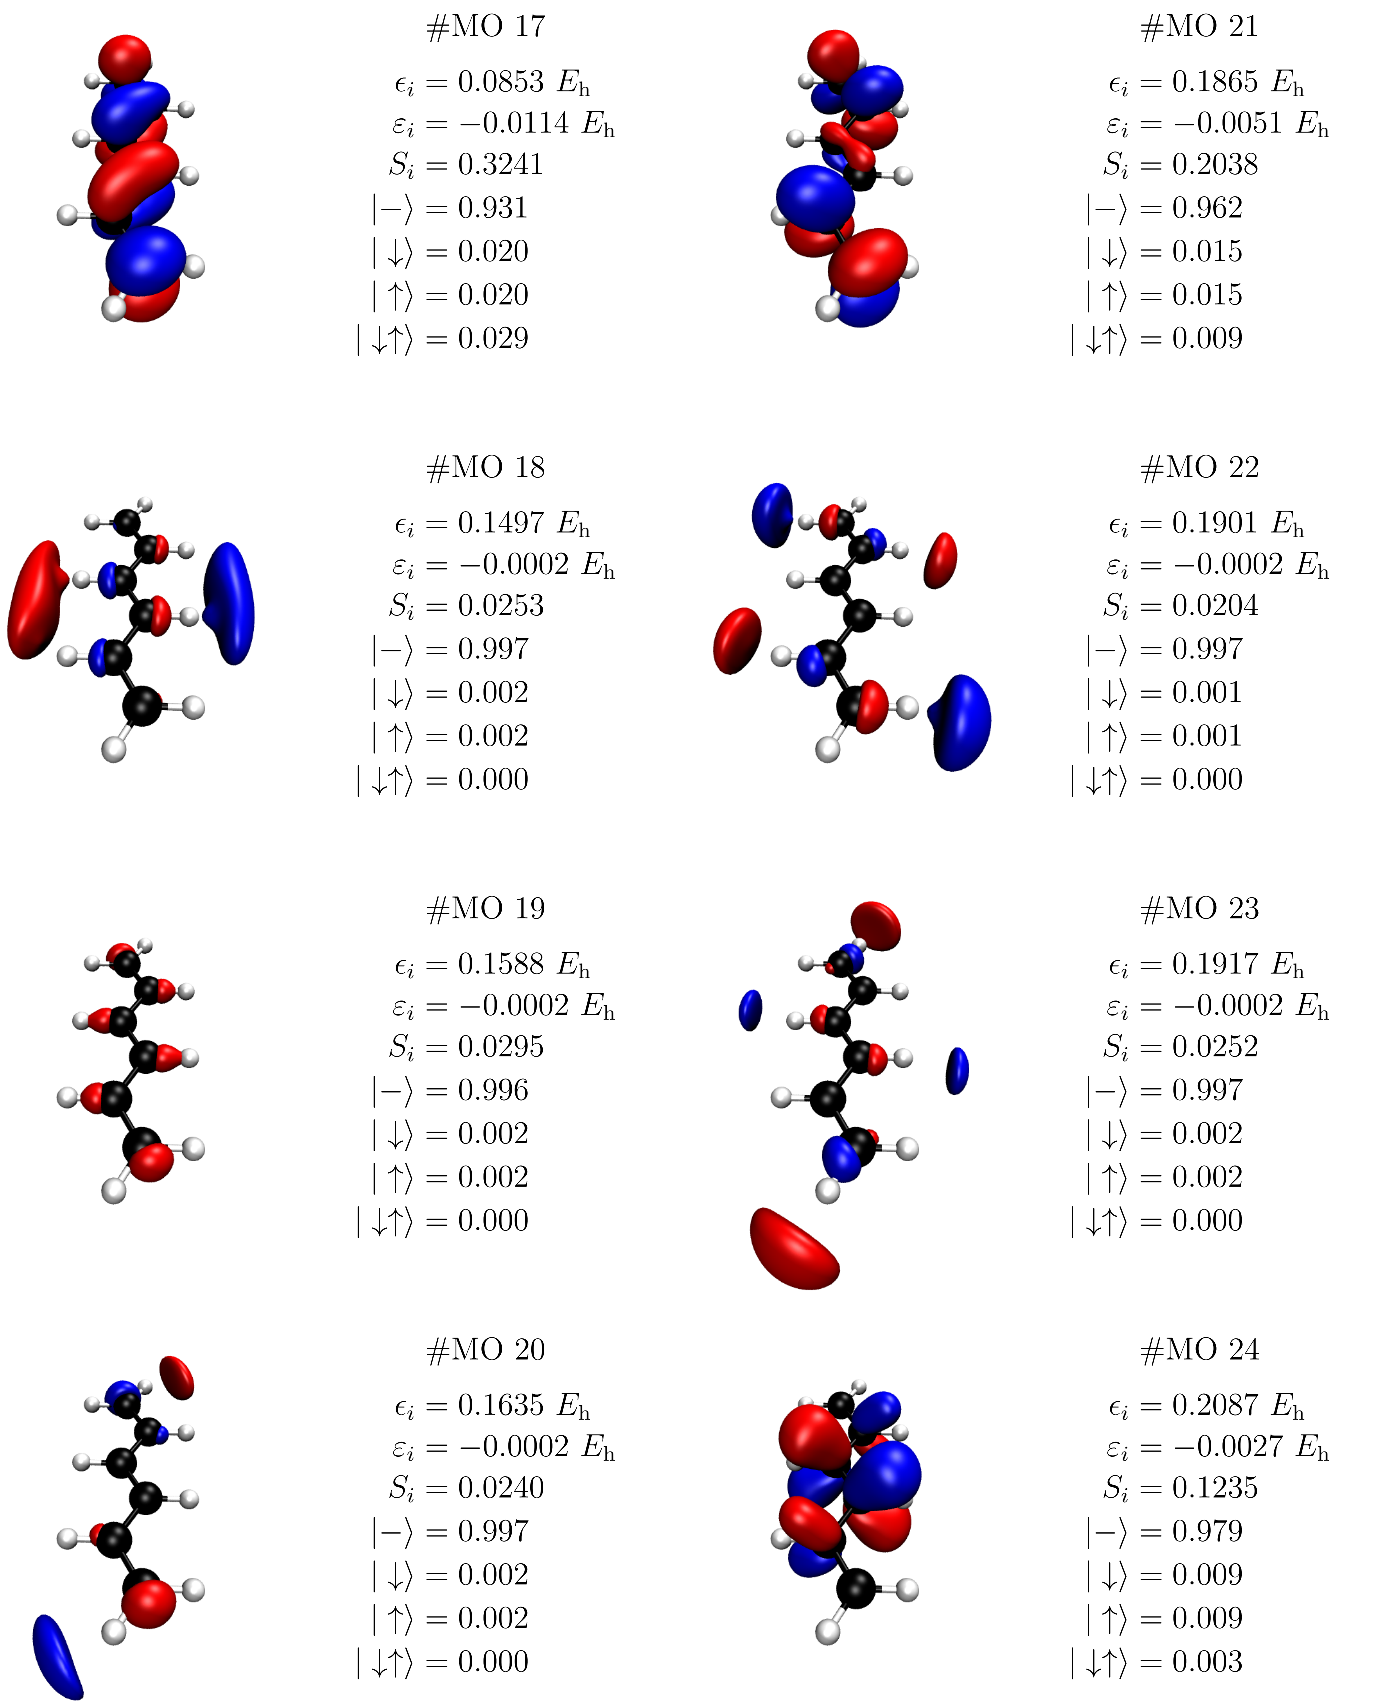


FIG. S3. Polyacetelene: Pipek-Mezey localized active space molecular orbitals #17 to #24 with their corresponding diagonal Fock matrix element $\epsilon_i$, 1-orbital increment $\varepsilon_i$, 1-orbital entropy $S_i$ and orbital occupations $\omega_{i,\alpha} = \{|-\rangle, |\downarrow\rangle, |\uparrow\rangle, |\downarrow\uparrow\rangle\}$. Isosurfaces are plotted at $|\psi(\vec{r})| = 0.05\ a_0^{-1.5}$).

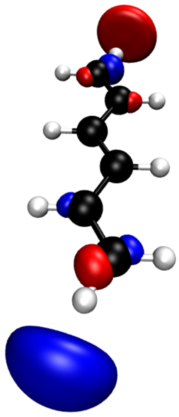

#MO 25

$\epsilon_i = 0.2205\ E_\mathrm{h}$
$\varepsilon_i = -0.0002\ E_\mathrm{h}$
$S_i = 0.0222$
$|-\rangle = 0.997$
$|\downarrow\rangle = 0.001$
$|\uparrow\rangle = 0.001$
$|\downarrow\uparrow\rangle = 0.000$

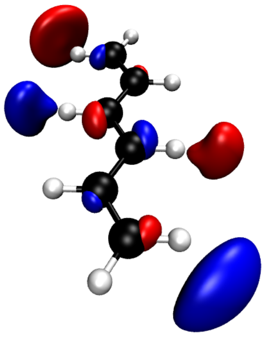

#MO 26

$\epsilon_i = 0.2471\ E_\mathrm{h}$
$\varepsilon_i = -0.0002\ E_\mathrm{h}$
$S_i = 0.0179$
$|-\rangle = 0.998$
$|\downarrow\rangle = 0.001$
$|\uparrow\rangle = 0.001$
$|\downarrow\uparrow\rangle = 0.000$

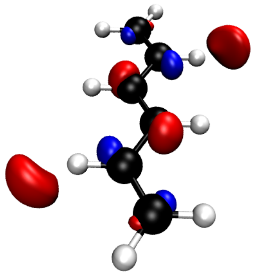

#MO 27

$\epsilon_i = 0.2592\ E_\mathrm{h}$
$\varepsilon_i = -0.0002\ E_\mathrm{h}$
$S_i = 0.0225$
$|-\rangle = 0.997$
$|\downarrow\rangle = 0.001$
$|\uparrow\rangle = 0.001$
$|\downarrow\uparrow\rangle = 0.000$

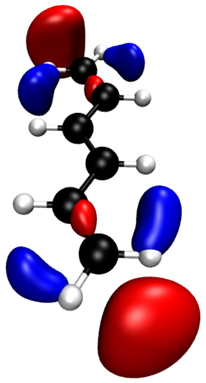

#MO 28

$\epsilon_i = 0.3109\ E_\mathrm{h}$
$\varepsilon_i = -0.0002\ E_\mathrm{h}$
$S_i = 0.0160$
$|-\rangle = 0.998$
$|\downarrow\rangle = 0.001$
$|\uparrow\rangle = 0.001$
$|\downarrow\uparrow\rangle = 0.000$

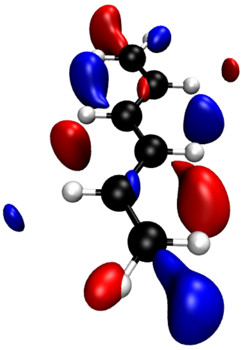

#MO 29

$\epsilon_i = 0.3524\ E_\mathrm{h}$
$\varepsilon_i = -0.0002\ E_\mathrm{h}$
$S_i = 0.0182$
$|-\rangle = 0.998$
$|\downarrow\rangle = 0.001$
$|\uparrow\rangle = 0.001$
$|\downarrow\uparrow\rangle = 0.000$

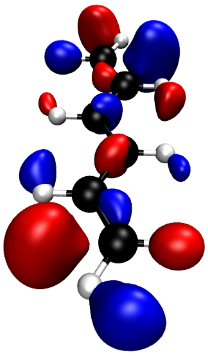

#MO 30

$\epsilon_i = 0.3771\ E_\mathrm{h}$
$\varepsilon_i = -0.0004\ E_\mathrm{h}$
$S_i = 0.0231$
$|-\rangle = 0.997$
$|\downarrow\rangle = 0.001$
$|\uparrow\rangle = 0.001$
$|\downarrow\uparrow\rangle = 0.000$

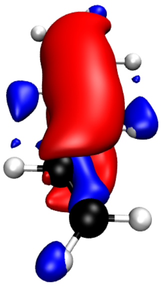

#MO 31

$\epsilon_i = 0.4203\ E_\mathrm{h}$
$\varepsilon_i = -0.0008\ E_\mathrm{h}$
$S_i = 0.0289$
$|-\rangle = 0.996$
$|\downarrow\rangle = 0.002$
$|\uparrow\rangle = 0.002$
$|\downarrow\uparrow\rangle = 0.000$

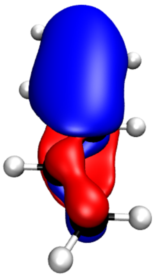

#MO 32

$\epsilon_i = 0.4275\ E_\mathrm{h}$
$\varepsilon_i = -0.0007\ E_\mathrm{h}$
$S_i = 0.0291$
$|-\rangle = 0.996$
$|\downarrow\rangle = 0.002$
$|\uparrow\rangle = 0.002$
$|\downarrow\uparrow\rangle = 0.000$

FIG. S4. Polyacetelene: Pipek-Mezey localized active space molecular orbitals #25 to #32 with their corresponding diagonal Fock matrix element $\epsilon_i$, 1-orbital increment $\varepsilon_i$, 1-orbital entropy $S_i$ and orbital occupations $\omega_{i,\alpha} = \{|-\rangle, |\downarrow\rangle, |\uparrow\rangle, |\downarrow\uparrow\rangle\}$. Isosurfaces are plotted at $|\psi(\vec{r})| = 0.05\ a_0^{-1.5}$).

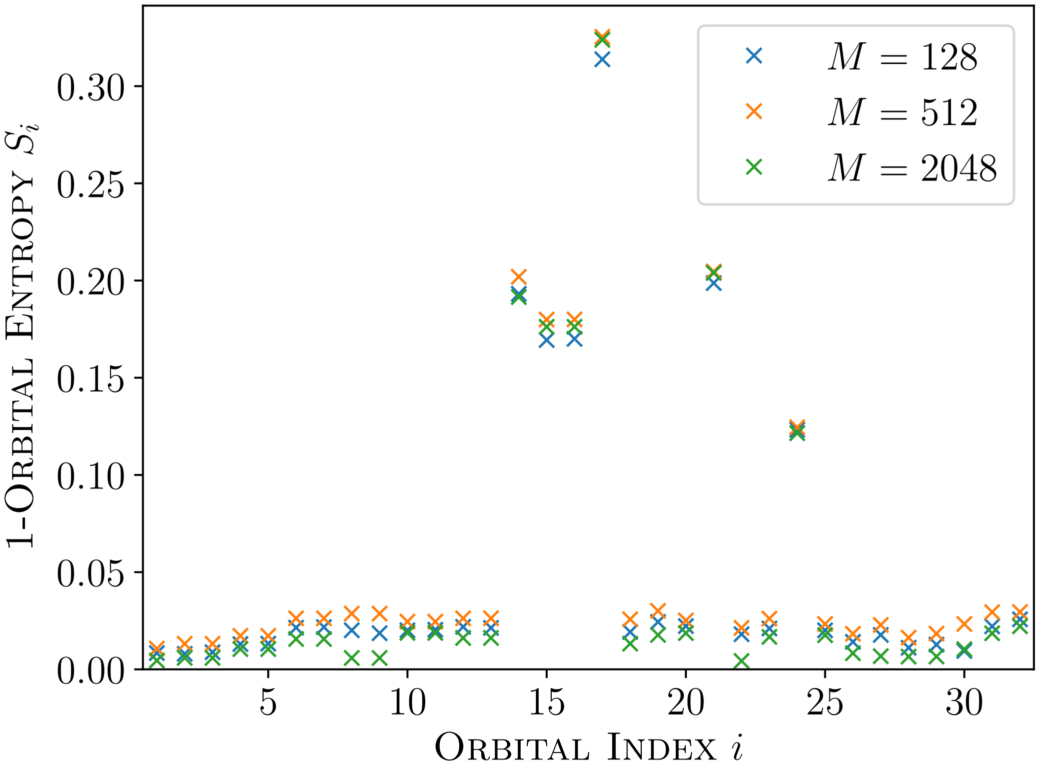


FIG. S5. Polyacetelene: Dependance of the 1-orbital entropies $S_i$ of the number of blockstates $M$ for an optimized orbital ordering.

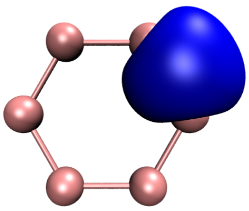

#MO 1

$\epsilon_i = -0.3291\ E_\mathrm{h}$
$\varepsilon_i = -0.0316\ E_\mathrm{h}$
$S_i = 0.2513$
$|-\rangle = 0.027$
$|\downarrow\rangle = 0.012$
$|\uparrow\rangle = 0.012$
$|\downarrow\uparrow\rangle = 0.949$

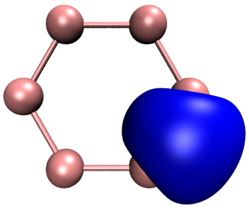

#MO 2

$\epsilon_i = -0.3291\ E_\mathrm{h}$
$\varepsilon_i = -0.0316\ E_\mathrm{h}$
$S_i = 0.2509$
$|-\rangle = 0.027$
$|\downarrow\rangle = 0.012$
$|\uparrow\rangle = 0.012$
$|\downarrow\uparrow\rangle = 0.950$

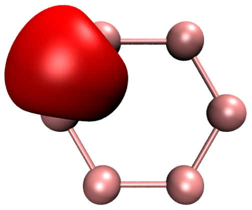

#MO 3

$\epsilon_i = -0.3291\ E_\mathrm{h}$
$\varepsilon_i = -0.0316\ E_\mathrm{h}$
$S_i = 0.2510$
$|-\rangle = 0.027$
$|\downarrow\rangle = 0.012$
$|\uparrow\rangle = 0.012$
$|\downarrow\uparrow\rangle = 0.950$

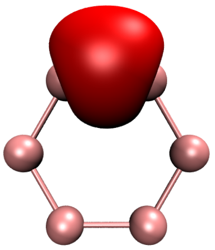

#MO 4

$\epsilon_i = -0.3291\ E_\mathrm{h}$
$\varepsilon_i = -0.0316\ E_\mathrm{h}$
$S_i = 0.2504$
$|-\rangle = 0.027$
$|\downarrow\rangle = 0.012$
$|\uparrow\rangle = 0.012$
$|\downarrow\uparrow\rangle = 0.950$

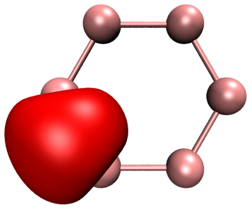

#MO 5

$\epsilon_i = -0.3291\ E_\mathrm{h}$
$\varepsilon_i = -0.0316\ E_\mathrm{h}$
$S_i = 0.2512$
$|-\rangle = 0.027$
$|\downarrow\rangle = 0.012$
$|\uparrow\rangle = 0.012$
$|\downarrow\uparrow\rangle = 0.950$

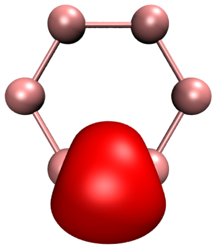

#MO 6

$\epsilon_i = -0.3291\ E_\mathrm{h}$
$\varepsilon_i = -0.0316\ E_\mathrm{h}$
$S_i = 0.2504$
$|-\rangle = 0.027$
$|\downarrow\rangle = 0.012$
$|\uparrow\rangle = 0.012$
$|\downarrow\uparrow\rangle = 0.950$

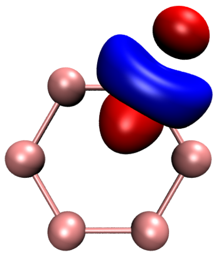

#MO 7

$\epsilon_i = 0.6138\ E_\mathrm{h}$
$\varepsilon_i = -0.0015\ E_\mathrm{h}$
$S_i = 0.0660$
$|-\rangle = 0.990$
$|\downarrow\rangle = 0.004$
$|\uparrow\rangle = 0.004$
$|\downarrow\uparrow\rangle = 0.002$

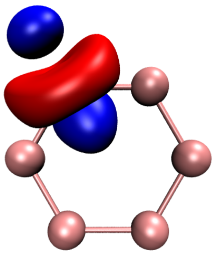

#MO 8

$\epsilon_i = 0.6138\ E_\mathrm{h}$
$\varepsilon_i = -0.0015\ E_\mathrm{h}$
$S_i = 0.0658$
$|-\rangle = 0.990$
$|\downarrow\rangle = 0.004$
$|\uparrow\rangle = 0.004$
$|\downarrow\uparrow\rangle = 0.002$

FIG. S6. $Be_6$ $R = 2.2$ Å: Foster-Boys localized active space molecular orbitals #1 to #8 with their corresponding diagonal Fock matrix element $\epsilon_i$, 1-orbital increment $\varepsilon_i$, 1-orbital entropy $S_i$ and orbital occupations $\omega_{i,\alpha} = \{|-\rangle, |\downarrow\rangle, |\uparrow\rangle, |\downarrow\uparrow\rangle\}$. Isosurfaces are plotted at $|\psi(\vec{r})| = 0.05\ a_0^{-1.5}$).

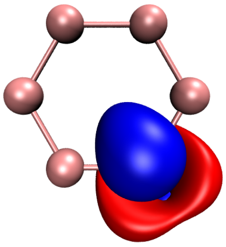

#MO 9

$\epsilon_i = 0.6153\ E_\mathrm{h}$
$\varepsilon_i = -0.0015\ E_\mathrm{h}$
$S_i = 0.0655$
$|-\rangle = 0.990$
$|\downarrow\rangle = 0.004$
$|\uparrow\rangle = 0.004$
$|\downarrow\uparrow\rangle = 0.002$

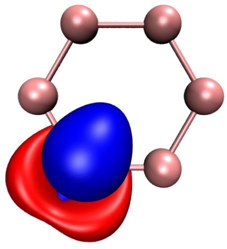

#MO 10

$\epsilon_i = 0.6153\ E_\mathrm{h}$
$\varepsilon_i = -0.0015\ E_\mathrm{h}$
$S_i = 0.0657$
$|-\rangle = 0.990$
$|\downarrow\rangle = 0.004$
$|\uparrow\rangle = 0.004$
$|\downarrow\uparrow\rangle = 0.002$

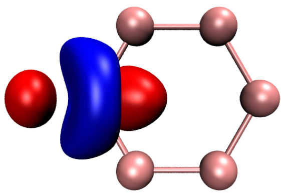

#MO 11

$\epsilon_i = 0.6155\ E_\mathrm{h}$
$\varepsilon_i = -0.0015\ E_\mathrm{h}$
$S_i = 0.0660$
$|-\rangle = 0.990$
$|\downarrow\rangle = 0.004$
$|\uparrow\rangle = 0.004$
$|\downarrow\uparrow\rangle = 0.002$

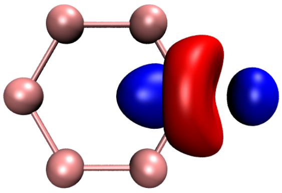

#MO 12

$\epsilon_i = 0.6155\ E_\mathrm{h}$
$\varepsilon_i = -0.0015\ E_\mathrm{h}$
$S_i = 0.0660$
$|-\rangle = 0.990$
$|\downarrow\rangle = 0.004$
$|\uparrow\rangle = 0.004$
$|\downarrow\uparrow\rangle = 0.002$

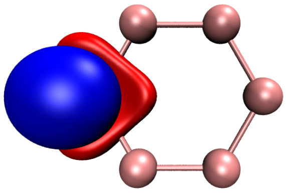

#MO 13

$\epsilon_i = 0.6239\ E_\mathrm{h}$
$\varepsilon_i = -0.0008\ E_\mathrm{h}$
$S_i = 0.0493$
$|-\rangle = 0.993$
$|\downarrow\rangle = 0.003$
$|\uparrow\rangle = 0.003$
$|\downarrow\uparrow\rangle = 0.001$

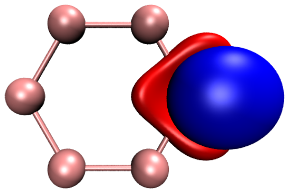

#MO 14

$\epsilon_i = 0.6239\ E_\mathrm{h}$
$\varepsilon_i = -0.0008\ E_\mathrm{h}$
$S_i = 0.0493$
$|-\rangle = 0.993$
$|\downarrow\rangle = 0.003$
$|\uparrow\rangle = 0.003$
$|\downarrow\uparrow\rangle = 0.001$

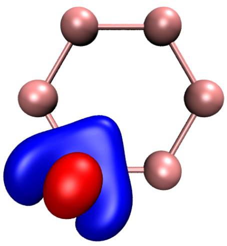

#MO 15

$\epsilon_i = 0.6241\ E_\mathrm{h}$
$\varepsilon_i = -0.0008\ E_\mathrm{h}$
$S_i = 0.0490$
$|-\rangle = 0.993$
$|\downarrow\rangle = 0.003$
$|\uparrow\rangle = 0.003$
$|\downarrow\uparrow\rangle = 0.001$

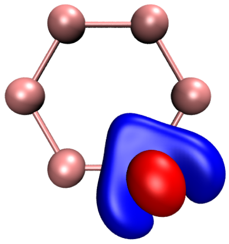

#MO 16

$\epsilon_i = 0.6241\ E_\mathrm{h}$
$\varepsilon_i = -0.0008\ E_\mathrm{h}$
$S_i = 0.0489$
$|-\rangle = 0.993$
$|\downarrow\rangle = 0.003$
$|\uparrow\rangle = 0.003$
$|\downarrow\uparrow\rangle = 0.001$

FIG. S7. $Be_6$ $R = 2.2$ Å: Foster-Boys localized active space molecular orbitals #9 to #16 with their corresponding diagonal Fock matrix element $\epsilon_i$, 1-orbital increment $\varepsilon_i$, 1-orbital entropy $S_i$ and orbital occupations $\omega_{i,\alpha} = \{|-\rangle, |\downarrow\rangle, |\uparrow\rangle, |\downarrow\uparrow\rangle\}$. Isosurfaces are plotted at $|\psi(\vec{r})| = 0.05\ a_0^{-1.5}$).

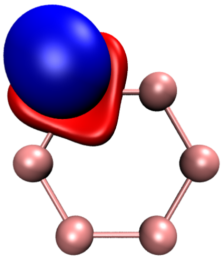

#MO 17

$\epsilon_i = 0.6246\ E_\mathrm{h}$
$\varepsilon_i = -0.0008\ E_\mathrm{h}$
$S_i = 0.0486$
$|{-}\rangle = 0.993$
$|{\downarrow}\rangle = 0.003$
$|{\uparrow}\rangle = 0.003$
$|{\downarrow\uparrow}\rangle = 0.001$

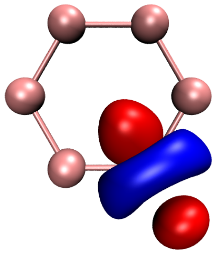

#MO 21

$\epsilon_i = 0.6388\ E_\mathrm{h}$
$\varepsilon_i = -0.0014\ E_\mathrm{h}$
$S_i = 0.0661$
$|{-}\rangle = 0.990$
$|{\downarrow}\rangle = 0.004$
$|{\uparrow}\rangle = 0.004$
$|{\downarrow\uparrow}\rangle = 0.002$

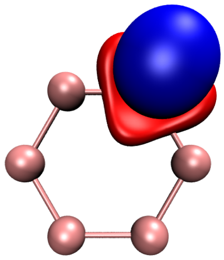

#MO 18

$\epsilon_i = 0.6246\ E_\mathrm{h}$
$\varepsilon_i = -0.0008\ E_\mathrm{h}$
$S_i = 0.0487$
$|{-}\rangle = 0.993$
$|{\downarrow}\rangle = 0.003$
$|{\uparrow}\rangle = 0.003$
$|{\downarrow\uparrow}\rangle = 0.001$

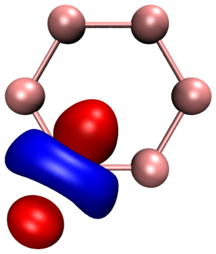

#MO 22

$\epsilon_i = 0.6388\ E_\mathrm{h}$
$\varepsilon_i = -0.0014\ E_\mathrm{h}$
$S_i = 0.0662$
$|{-}\rangle = 0.990$
$|{\downarrow}\rangle = 0.004$
$|{\uparrow}\rangle = 0.004$
$|{\downarrow\uparrow}\rangle = 0.002$

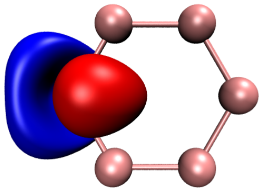

#MO 19

$\epsilon_i = 0.6387\ E_\mathrm{h}$
$\varepsilon_i = -0.0014\ E_\mathrm{h}$
$S_i = 0.0665$
$|{-}\rangle = 0.990$
$|{\downarrow}\rangle = 0.004$
$|{\uparrow}\rangle = 0.004$
$|{\downarrow\uparrow}\rangle = 0.002$

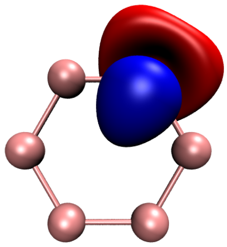

#MO 23

$\epsilon_i = 0.6399\ E_\mathrm{h}$
$\varepsilon_i = -0.0014\ E_\mathrm{h}$
$S_i = 0.0660$
$|{-}\rangle = 0.990$
$|{\downarrow}\rangle = 0.004$
$|{\uparrow}\rangle = 0.004$
$|{\downarrow\uparrow}\rangle = 0.002$

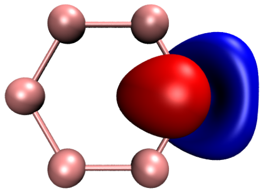

#MO 20

$\epsilon_i = 0.6387\ E_\mathrm{h}$
$\varepsilon_i = -0.0014\ E_\mathrm{h}$
$S_i = 0.0665$
$|{-}\rangle = 0.990$
$|{\downarrow}\rangle = 0.004$
$|{\uparrow}\rangle = 0.004$
$|{\downarrow\uparrow}\rangle = 0.002$

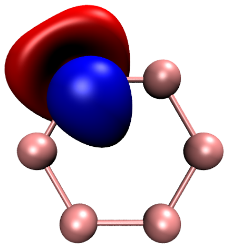

#MO 24

$\epsilon_i = 0.6399\ E_\mathrm{h}$
$\varepsilon_i = -0.0014\ E_\mathrm{h}$
$S_i = 0.0658$
$|{-}\rangle = 0.990$
$|{\downarrow}\rangle = 0.004$
$|{\uparrow}\rangle = 0.004$
$|{\downarrow\uparrow}\rangle = 0.002$

FIG. S8. $Be_6$ $R = 2.2$ Å: Foster-Boys localized active space molecular orbitals #17 to #24 with their corresponding diagonal Fock matrix element $\epsilon_i$, 1-orbital increment $\varepsilon_i$, 1-orbital entropy $S_i$ and orbital occupations $\omega_{i,\alpha} = \{|{-}\rangle, |{\downarrow}\rangle, |{\uparrow}\rangle, |{\downarrow\uparrow}\rangle\}$. Isosurfaces are plotted at $|\psi(\vec{r})| = 0.05\ a_0^{-1.5}$).

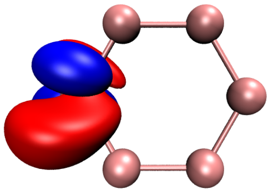

#MO 25

$\epsilon_i = 0.6463\ E_\mathrm{h}$

$\varepsilon_i = -0.0013\ E_\mathrm{h}$

$S_i = 0.0494$

$|{-}\rangle = 0.993$

$|\downarrow\rangle = 0.003$

$|\uparrow\rangle = 0.003$

$|\downarrow\uparrow\rangle = 0.001$

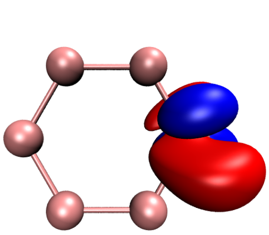

#MO 26

$\epsilon_i = 0.6463\ E_\mathrm{h}$

$\varepsilon_i = -0.0013\ E_\mathrm{h}$

$S_i = 0.0493$

$|{-}\rangle = 0.993$

$|\downarrow\rangle = 0.003$

$|\uparrow\rangle = 0.003$

$|\downarrow\uparrow\rangle = 0.001$

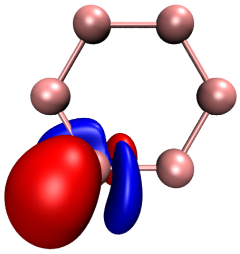

#MO 27

$\epsilon_i = 0.6477\ E_\mathrm{h}$

$\varepsilon_i = -0.0013\ E_\mathrm{h}$

$S_i = 0.0491$

$|{-}\rangle = 0.993$

$|\downarrow\rangle = 0.003$

$|\uparrow\rangle = 0.003$

$|\downarrow\uparrow\rangle = 0.001$

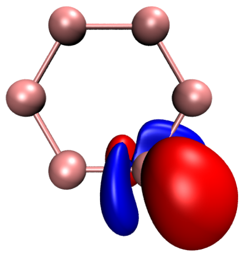

#MO 28

$\epsilon_i = 0.6477\ E_\mathrm{h}$

$\varepsilon_i = -0.0013\ E_\mathrm{h}$

$S_i = 0.0490$

$|{-}\rangle = 0.993$

$|\downarrow\rangle = 0.003$

$|\uparrow\rangle = 0.003$

$|\downarrow\uparrow\rangle = 0.001$

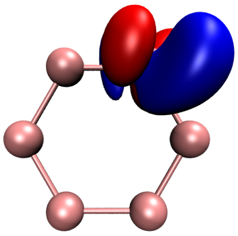

#MO 29

$\epsilon_i = 0.6516\ E_\mathrm{h}$

$\varepsilon_i = -0.0014\ E_\mathrm{h}$

$S_i = 0.0496$

$|{-}\rangle = 0.993$

$|\downarrow\rangle = 0.003$

$|\uparrow\rangle = 0.003$

$|\downarrow\uparrow\rangle = 0.001$

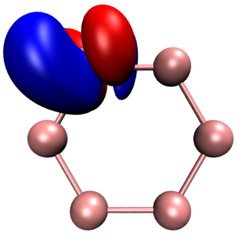

#MO 30

$\epsilon_i = 0.6516\ E_\mathrm{h}$

$\varepsilon_i = -0.0014\ E_\mathrm{h}$

$S_i = 0.0496$

$|{-}\rangle = 0.993$

$|\downarrow\rangle = 0.003$

$|\uparrow\rangle = 0.003$

$|\downarrow\uparrow\rangle = 0.001$

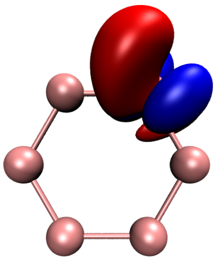

#MO 31

$\epsilon_i = 0.6531\ E_\mathrm{h}$

$\varepsilon_i = -0.0014\ E_\mathrm{h}$

$S_i = 0.0494$

$|{-}\rangle = 0.993$

$|\downarrow\rangle = 0.003$

$|\uparrow\rangle = 0.003$

$|\downarrow\uparrow\rangle = 0.001$

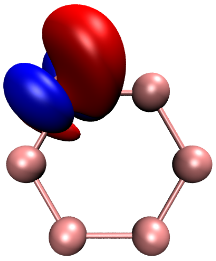

#MO 32

$\epsilon_i = 0.6531\ E_\mathrm{h}$

$\varepsilon_i = -0.0014\ E_\mathrm{h}$

$S_i = 0.0493$

$|{-}\rangle = 0.993$

$|\downarrow\rangle = 0.003$

$|\uparrow\rangle = 0.003$

$|\downarrow\uparrow\rangle = 0.001$

FIG. S9. $Be_6$ $R = 2.2$ Å: Foster-Boys localized active space molecular orbitals #25 to #32 with their corresponding diagonal Fock matrix element $\epsilon_i$, 1-orbital increment $\varepsilon_i$, 1-orbital entropy $S_i$ and orbital occupations $\omega_{i,\alpha} = \{|{-}\rangle, |\downarrow\rangle, |\uparrow\rangle, |\downarrow\uparrow\rangle\}$. Isosurfaces are plotted at $|\psi(\vec{r})| = 0.05\ a_0^{-1.5}$).

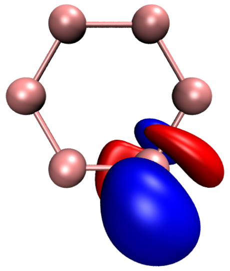

#MO 33

$\epsilon_i = 0.6594\ E_\mathrm{h}$
$\varepsilon_i = -0.0015\ E_\mathrm{h}$
$S_i = 0.0492$
$|-\rangle = 0.993$
$|\downarrow\rangle = 0.003$
$|\uparrow\rangle = 0.003$
$|\downarrow\uparrow\rangle = 0.001$

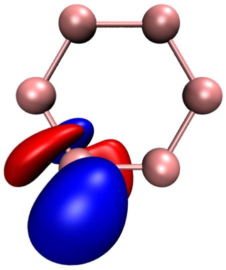

#MO 34

$\epsilon_i = 0.6595\ E_\mathrm{h}$
$\varepsilon_i = -0.0015\ E_\mathrm{h}$
$S_i = 0.0493$
$|-\rangle = 0.993$
$|\downarrow\rangle = 0.003$
$|\uparrow\rangle = 0.003$
$|\downarrow\uparrow\rangle = 0.001$

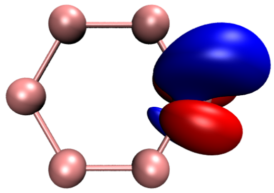

#MO 35

$\epsilon_i = 0.6609\ E_\mathrm{h}$
$\varepsilon_i = -0.0015\ E_\mathrm{h}$
$S_i = 0.0495$
$|-\rangle = 0.993$
$|\downarrow\rangle = 0.003$
$|\uparrow\rangle = 0.003$
$|\downarrow\uparrow\rangle = 0.001$

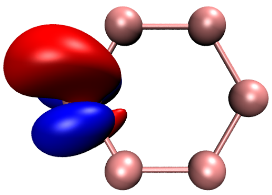

#MO 36

$\epsilon_i = 0.6609\ E_\mathrm{h}$
$\varepsilon_i = -0.0015\ E_\mathrm{h}$
$S_i = 0.0495$
$|-\rangle = 0.993$
$|\downarrow\rangle = 0.003$
$|\uparrow\rangle = 0.003$
$|\downarrow\uparrow\rangle = 0.001$

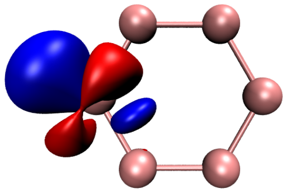

#MO 37

$\epsilon_i = 0.6878\ E_\mathrm{h}$
$\varepsilon_i = -0.0011\ E_\mathrm{h}$
$S_i = 0.0459$
$|-\rangle = 0.994$
$|\downarrow\rangle = 0.003$
$|\uparrow\rangle = 0.003$
$|\downarrow\uparrow\rangle = 0.001$

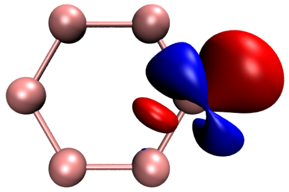

#MO 38

$\epsilon_i = 0.6878\ E_\mathrm{h}$
$\varepsilon_i = -0.0011\ E_\mathrm{h}$
$S_i = 0.0459$
$|-\rangle = 0.994$
$|\downarrow\rangle = 0.003$
$|\uparrow\rangle = 0.003$
$|\downarrow\uparrow\rangle = 0.001$

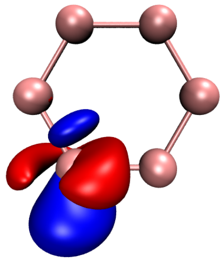

#MO 39

$\epsilon_i = 0.6881\ E_\mathrm{h}$
$\varepsilon_i = -0.0011\ E_\mathrm{h}$
$S_i = 0.0455$
$|-\rangle = 0.994$
$|\downarrow\rangle = 0.003$
$|\uparrow\rangle = 0.003$
$|\downarrow\uparrow\rangle = 0.001$

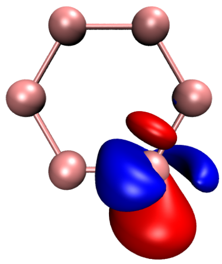

#MO 40

$\epsilon_i = 0.6881\ E_\mathrm{h}$
$\varepsilon_i = -0.0011\ E_\mathrm{h}$
$S_i = 0.0455$
$|-\rangle = 0.994$
$|\downarrow\rangle = 0.003$
$|\uparrow\rangle = 0.003$
$|\downarrow\uparrow\rangle = 0.001$

FIG. S10. $Be_6$ $R = 2.2$ Å: Foster-Boys localized active space molecular orbitals #33 to #40 with their corresponding diagonal Fock matrix element $\epsilon_i$, 1-orbital increment $\varepsilon_i$, 1-orbital entropy $S_i$ and orbital occupations $\omega_{i,\alpha} = \{|-\rangle, |\downarrow\rangle, |\uparrow\rangle, |\downarrow\uparrow\rangle\}$. Isosurfaces are plotted at $|\psi(\vec{r})| = 0.05\ a_0^{-1.5}$).

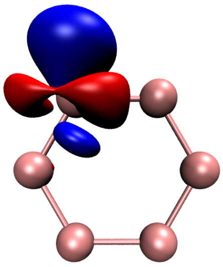

#MO 41

$\epsilon_i = 0.6906\ E_\mathrm{h}$

$\varepsilon_i = -0.0011\ E_\mathrm{h}$

$S_i = 0.0454$

$|-\rangle = 0.994$

$|\downarrow\rangle = 0.003$

$|\uparrow\rangle = 0.003$

$|\downarrow\uparrow\rangle = 0.001$

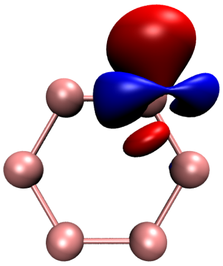

#MO 42

$\epsilon_i = 0.6906\ E_\mathrm{h}$

$\varepsilon_i = -0.0011\ E_\mathrm{h}$

$S_i = 0.0454$

$|-\rangle = 0.994$

$|\downarrow\rangle = 0.003$

$|\uparrow\rangle = 0.003$

$|\downarrow\uparrow\rangle = 0.001$

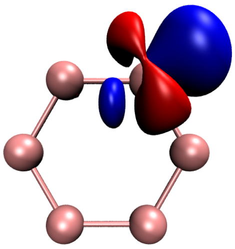

#MO 43

$\epsilon_i = 0.6910\ E_\mathrm{h}$

$\varepsilon_i = -0.0011\ E_\mathrm{h}$

$S_i = 0.0457$

$|-\rangle = 0.994$

$|\downarrow\rangle = 0.003$

$|\uparrow\rangle = 0.003$

$|\downarrow\uparrow\rangle = 0.001$

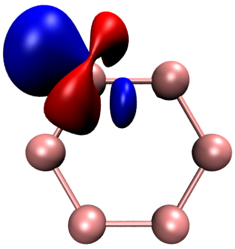

#MO 44

$\epsilon_i = 0.6910\ E_\mathrm{h}$

$\varepsilon_i = -0.0011\ E_\mathrm{h}$

$S_i = 0.0456$

$|-\rangle = 0.994$

$|\downarrow\rangle = 0.003$

$|\uparrow\rangle = 0.003$

$|\downarrow\uparrow\rangle = 0.001$

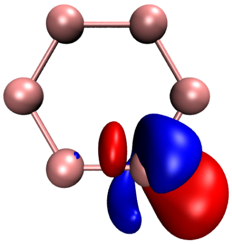

#MO 45

$\epsilon_i = 0.6913\ E_\mathrm{h}$

$\varepsilon_i = -0.0011\ E_\mathrm{h}$

$S_i = 0.0457$

$|-\rangle = 0.994$

$|\downarrow\rangle = 0.003$

$|\uparrow\rangle = 0.003$

$|\downarrow\uparrow\rangle = 0.001$

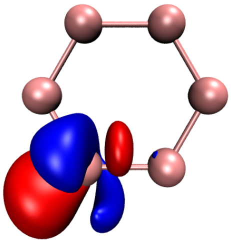

#MO 46

$\epsilon_i = 0.6913\ E_\mathrm{h}$

$\varepsilon_i = -0.0011\ E_\mathrm{h}$

$S_i = 0.0458$

$|-\rangle = 0.994$

$|\downarrow\rangle = 0.003$

$|\uparrow\rangle = 0.003$

$|\downarrow\uparrow\rangle = 0.001$

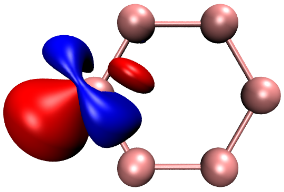

#MO 47

$\epsilon_i = 0.6916\ E_\mathrm{h}$

$\varepsilon_i = -0.0011\ E_\mathrm{h}$

$S_i = 0.0459$

$|-\rangle = 0.994$

$|\downarrow\rangle = 0.003$

$|\uparrow\rangle = 0.003$

$|\downarrow\uparrow\rangle = 0.001$

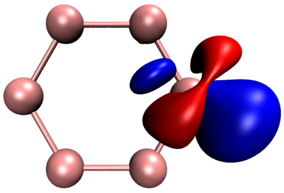

#MO 48

$\epsilon_i = 0.6916\ E_\mathrm{h}$

$\varepsilon_i = -0.0011\ E_\mathrm{h}$

$S_i = 0.0458$

$|-\rangle = 0.994$

$|\downarrow\rangle = 0.003$

$|\uparrow\rangle = 0.003$

$|\downarrow\uparrow\rangle = 0.001$

FIG. S11. $Be_6$ $R = 2.2$ Å: Foster-Boys localized active space molecular orbitals #41 to #48 with their corresponding diagonal Fock matrix element $\epsilon_i$, 1-orbital increment $\varepsilon_i$, 1-orbital entropy $S_i$ and orbital occupations $\omega_{i,\alpha} = \{|-\rangle, |\downarrow\rangle, |\uparrow\rangle, |\downarrow\uparrow\rangle\}$. Isosurfaces are plotted at $|\psi(\vec{r})| = 0.05\ a_0^{-1.5}$).

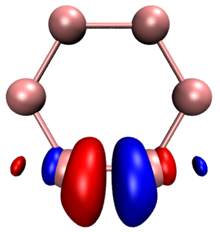

#MO 49

$\epsilon_i = 0.8201\ E_\mathrm{h}$
$\varepsilon_i = -0.0043\ E_\mathrm{h}$
$S_i = 0.0680$
$|-\rangle = 0.990$
$|\downarrow\rangle = 0.003$
$|\uparrow\rangle = 0.003$
$|\downarrow\uparrow\rangle = 0.004$

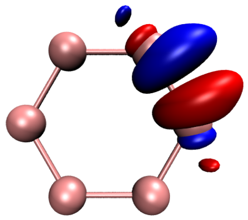

#MO 50

$\epsilon_i = 0.8216\ E_\mathrm{h}$
$\varepsilon_i = -0.0043\ E_\mathrm{h}$
$S_i = 0.0682$
$|-\rangle = 0.990$
$|\downarrow\rangle = 0.003$
$|\uparrow\rangle = 0.003$
$|\downarrow\uparrow\rangle = 0.004$

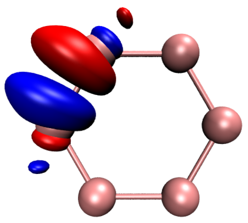

#MO 51

$\epsilon_i = 0.8216\ E_\mathrm{h}$
$\varepsilon_i = -0.0043\ E_\mathrm{h}$
$S_i = 0.0681$
$|-\rangle = 0.990$
$|\downarrow\rangle = 0.003$
$|\uparrow\rangle = 0.003$
$|\downarrow\uparrow\rangle = 0.004$

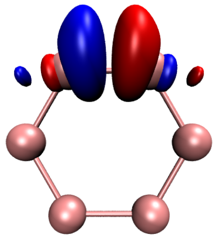

#MO 52

$\epsilon_i = 0.8230\ E_\mathrm{h}$
$\varepsilon_i = -0.0043\ E_\mathrm{h}$
$S_i = 0.0677$
$|-\rangle = 0.990$
$|\downarrow\rangle = 0.003$
$|\uparrow\rangle = 0.003$
$|\downarrow\uparrow\rangle = 0.004$

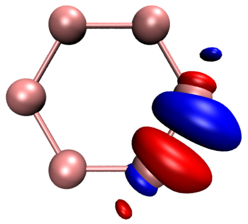

#MO 53

$\epsilon_i = 0.8252\ E_\mathrm{h}$
$\varepsilon_i = -0.0043\ E_\mathrm{h}$
$S_i = 0.0677$
$|-\rangle = 0.990$
$|\downarrow\rangle = 0.003$
$|\uparrow\rangle = 0.003$
$|\downarrow\uparrow\rangle = 0.004$

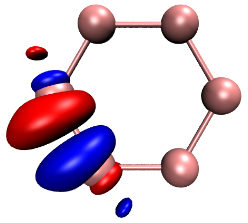

#MO 54

$\epsilon_i = 0.8252\ E_\mathrm{h}$
$\varepsilon_i = -0.0043\ E_\mathrm{h}$
$S_i = 0.0678$
$|-\rangle = 0.990$
$|\downarrow\rangle = 0.003$
$|\uparrow\rangle = 0.003$
$|\downarrow\uparrow\rangle = 0.004$

FIG. S12. $Be_6$ $R = 2.2$ Å: Foster-Boys localized active space molecular orbitals #49 to #54 with their corresponding diagonal Fock matrix element $\epsilon_i$, 1-orbital increment $\varepsilon_i$, 1-orbital entropy $S_i$ and orbital occupations $\omega_{i,\alpha} = \{|-\rangle, |\downarrow\rangle, |\uparrow\rangle, |\downarrow\uparrow\rangle\}$. Isosurfaces are plotted at $|\psi(\vec{r})| = 0.05\ a_0^{-1.5}$).

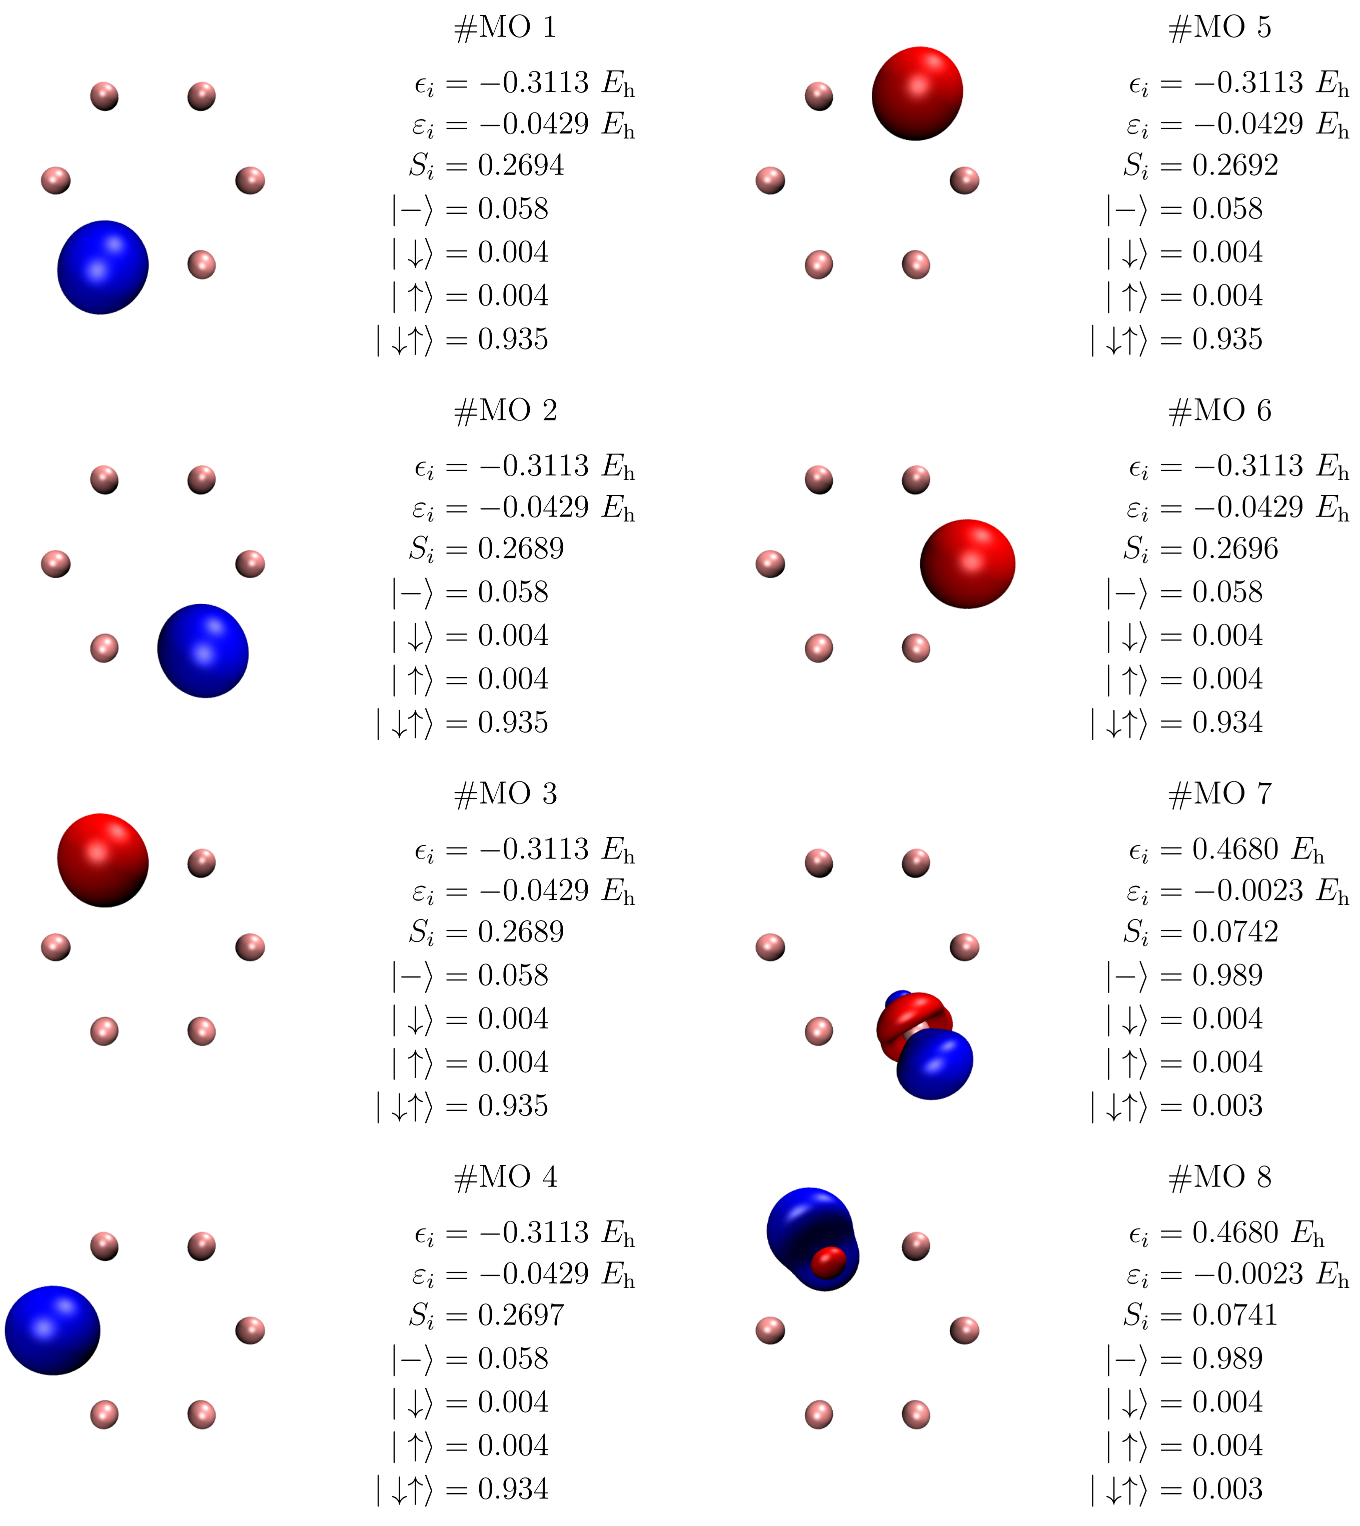


FIG. S13. $Be_6$ $R = 3.5$ Å: Foster-Boys localized active space molecular orbitals #1 to #8 with their corresponding diagonal Fock matrix element $\epsilon_i$, 1-orbital increment $\varepsilon_i$, 1-orbital entropy $S_i$ and orbital occupations $\omega_{i,\alpha} = \{|-\rangle, |\downarrow\rangle, |\uparrow\rangle, |\downarrow\uparrow\rangle\}$. Isosurfaces are plotted at $|\psi(\vec{r})| = 0.05\ a_0^{-1.5}$).

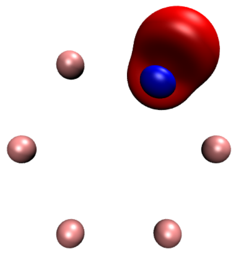

#MO 9

$\epsilon_i = 0.4680\ E_\mathrm{h}$
$\varepsilon_i = -0.0023\ E_\mathrm{h}$
$S_i = 0.0741$
$|{-}\rangle = 0.989$
$|\downarrow\rangle = 0.004$
$|\uparrow\rangle = 0.004$
$|\downarrow\uparrow\rangle = 0.003$

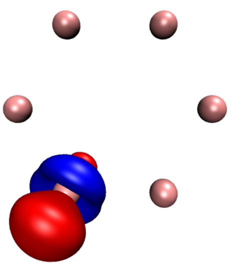

#MO 10

$\epsilon_i = 0.4680\ E_\mathrm{h}$
$\varepsilon_i = -0.0023\ E_\mathrm{h}$
$S_i = 0.0742$
$|{-}\rangle = 0.989$
$|\downarrow\rangle = 0.004$
$|\uparrow\rangle = 0.004$
$|\downarrow\uparrow\rangle = 0.003$

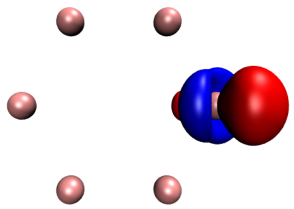

#MO 11

$\epsilon_i = 0.4680\ E_\mathrm{h}$
$\varepsilon_i = -0.0023\ E_\mathrm{h}$
$S_i = 0.0742$
$|{-}\rangle = 0.989$
$|\downarrow\rangle = 0.004$
$|\uparrow\rangle = 0.004$
$|\downarrow\uparrow\rangle = 0.003$

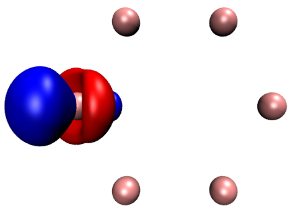

#MO 12

$\epsilon_i = 0.4680\ E_\mathrm{h}$
$\varepsilon_i = -0.0023\ E_\mathrm{h}$
$S_i = 0.0742$
$|{-}\rangle = 0.989$
$|\downarrow\rangle = 0.004$
$|\uparrow\rangle = 0.004$
$|\downarrow\uparrow\rangle = 0.003$

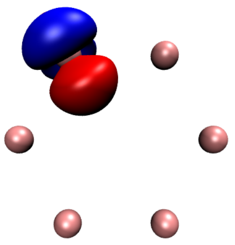

#MO 13

$\epsilon_i = 0.4726\ E_\mathrm{h}$
$\varepsilon_i = -0.0021\ E_\mathrm{h}$
$S_i = 0.0771$
$|{-}\rangle = 0.988$
$|\downarrow\rangle = 0.004$
$|\uparrow\rangle = 0.004$
$|\downarrow\uparrow\rangle = 0.003$

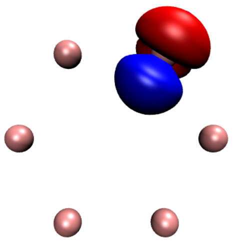

#MO 14

$\epsilon_i = 0.4726\ E_\mathrm{h}$
$\varepsilon_i = -0.0021\ E_\mathrm{h}$
$S_i = 0.0772$
$|{-}\rangle = 0.988$
$|\downarrow\rangle = 0.004$
$|\uparrow\rangle = 0.004$
$|\downarrow\uparrow\rangle = 0.003$

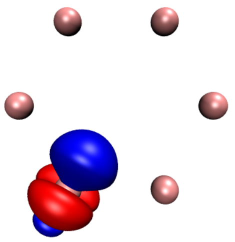

#MO 15

$\epsilon_i = 0.4726\ E_\mathrm{h}$
$\varepsilon_i = -0.0021\ E_\mathrm{h}$
$S_i = 0.0772$
$|{-}\rangle = 0.988$
$|\downarrow\rangle = 0.004$
$|\uparrow\rangle = 0.004$
$|\downarrow\uparrow\rangle = 0.003$

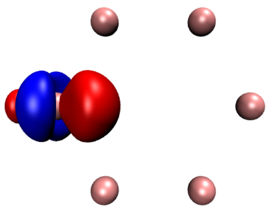

#MO 16

$\epsilon_i = 0.4726\ E_\mathrm{h}$
$\varepsilon_i = -0.0021\ E_\mathrm{h}$
$S_i = 0.0773$
$|{-}\rangle = 0.988$
$|\downarrow\rangle = 0.004$
$|\uparrow\rangle = 0.004$
$|\downarrow\uparrow\rangle = 0.003$

FIG. S14. $Be_6$ $R = 3.5$ Å: Foster-Boys localized active space molecular orbitals #9 to #16 with their corresponding diagonal Fock matrix element $\epsilon_i$, 1-orbital increment $\varepsilon_i$, 1-orbital entropy $S_i$ and orbital occupations $\omega_{i,\alpha} = \{|{-}\rangle, |\downarrow\rangle, |\uparrow\rangle, |\downarrow\uparrow\rangle\}$. Isosurfaces are plotted at $|\psi(\vec{r})| = 0.05\ a_0^{-1.5}$).

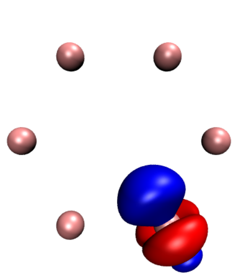

#MO 17

$\epsilon_i = 0.4726\ E_\mathrm{h}$
$\varepsilon_i = -0.0021\ E_\mathrm{h}$
$S_i = 0.0771$
$|-\rangle = 0.988$
$|\downarrow\rangle = 0.004$
$|\uparrow\rangle = 0.004$
$|\downarrow\uparrow\rangle = 0.003$

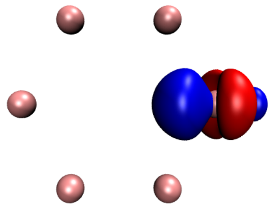

#MO 18

$\epsilon_i = 0.4726\ E_\mathrm{h}$
$\varepsilon_i = -0.0021\ E_\mathrm{h}$
$S_i = 0.0773$
$|-\rangle = 0.988$
$|\downarrow\rangle = 0.004$
$|\uparrow\rangle = 0.004$
$|\downarrow\uparrow\rangle = 0.003$

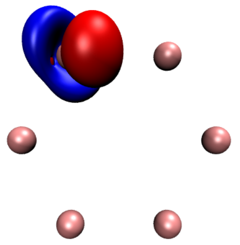

#MO 19

$\epsilon_i = 0.4824\ E_\mathrm{h}$
$\varepsilon_i = -0.0024\ E_\mathrm{h}$
$S_i = 0.0812$
$|-\rangle = 0.987$
$|\downarrow\rangle = 0.004$
$|\uparrow\rangle = 0.004$
$|\downarrow\uparrow\rangle = 0.004$

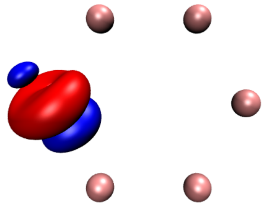

#MO 20

$\epsilon_i = 0.4824\ E_\mathrm{h}$
$\varepsilon_i = -0.0024\ E_\mathrm{h}$
$S_i = 0.0815$
$|-\rangle = 0.987$
$|\downarrow\rangle = 0.004$
$|\uparrow\rangle = 0.004$
$|\downarrow\uparrow\rangle = 0.004$

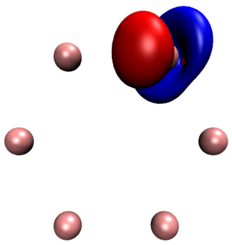

#MO 21

$\epsilon_i = 0.4824\ E_\mathrm{h}$
$\varepsilon_i = -0.0024\ E_\mathrm{h}$
$S_i = 0.0813$
$|-\rangle = 0.987$
$|\downarrow\rangle = 0.004$
$|\uparrow\rangle = 0.004$
$|\downarrow\uparrow\rangle = 0.004$

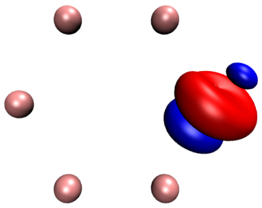

#MO 22

$\epsilon_i = 0.4824\ E_\mathrm{h}$
$\varepsilon_i = -0.0024\ E_\mathrm{h}$
$S_i = 0.0814$
$|-\rangle = 0.987$
$|\downarrow\rangle = 0.004$
$|\uparrow\rangle = 0.004$
$|\downarrow\uparrow\rangle = 0.004$

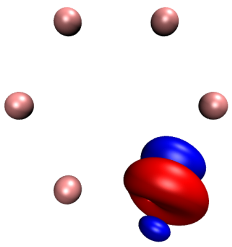

#MO 23

$\epsilon_i = 0.4825\ E_\mathrm{h}$
$\varepsilon_i = -0.0024\ E_\mathrm{h}$
$S_i = 0.0814$
$|-\rangle = 0.987$
$|\downarrow\rangle = 0.004$
$|\uparrow\rangle = 0.004$
$|\downarrow\uparrow\rangle = 0.004$

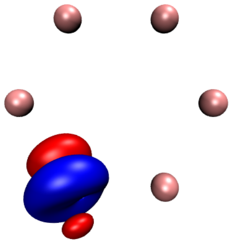

#MO 24

$\epsilon_i = 0.4825\ E_\mathrm{h}$
$\varepsilon_i = -0.0024\ E_\mathrm{h}$
$S_i = 0.0815$
$|-\rangle = 0.987$
$|\downarrow\rangle = 0.004$
$|\uparrow\rangle = 0.004$
$|\downarrow\uparrow\rangle = 0.004$

FIG. S15. $Be_6$ $R = 3.5$ Å: Foster-Boys localized active space molecular orbitals #17 to #24 with their corresponding diagonal Fock matrix element $\epsilon_i$, 1-orbital increment $\varepsilon_i$, 1-orbital entropy $S_i$ and orbital occupations $\omega_{i,\alpha} = \{|-\rangle, |\downarrow\rangle, |\uparrow\rangle, |\downarrow\uparrow\rangle\}$. Isosurfaces are plotted at $|\psi(\vec{r})| = 0.05\ a_0^{-1.5}$).

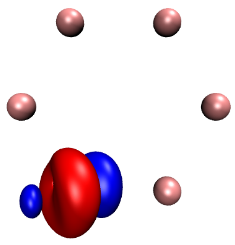

#MO 25

$\epsilon_i = 0.4825\ E_\mathrm{h}$
$\varepsilon_i = -0.0024\ E_\mathrm{h}$
$S_i = 0.0813$
$|-\rangle = 0.987$
$|\downarrow\rangle = 0.004$
$|\uparrow\rangle = 0.004$
$|\downarrow\uparrow\rangle = 0.004$

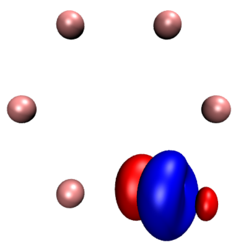

#MO 26

$\epsilon_i = 0.4825\ E_\mathrm{h}$
$\varepsilon_i = -0.0024\ E_\mathrm{h}$
$S_i = 0.0813$
$|-\rangle = 0.987$
$|\downarrow\rangle = 0.004$
$|\uparrow\rangle = 0.004$
$|\downarrow\uparrow\rangle = 0.004$

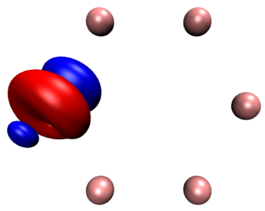

#MO 27

$\epsilon_i = 0.4827\ E_\mathrm{h}$
$\varepsilon_i = -0.0024\ E_\mathrm{h}$
$S_i = 0.0814$
$|-\rangle = 0.987$
$|\downarrow\rangle = 0.004$
$|\uparrow\rangle = 0.004$
$|\downarrow\uparrow\rangle = 0.004$

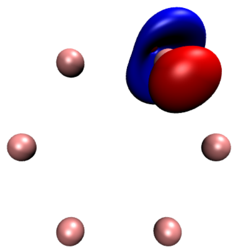

#MO 28

$\epsilon_i = 0.4827\ E_\mathrm{h}$
$\varepsilon_i = -0.0024\ E_\mathrm{h}$
$S_i = 0.0814$
$|-\rangle = 0.987$
$|\downarrow\rangle = 0.004$
$|\uparrow\rangle = 0.004$
$|\downarrow\uparrow\rangle = 0.004$

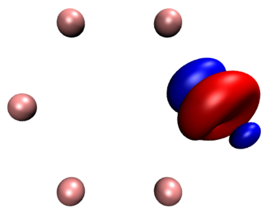

#MO 29

$\epsilon_i = 0.4827\ E_\mathrm{h}$
$\varepsilon_i = -0.0024\ E_\mathrm{h}$
$S_i = 0.0814$
$|-\rangle = 0.987$
$|\downarrow\rangle = 0.004$
$|\uparrow\rangle = 0.004$
$|\downarrow\uparrow\rangle = 0.004$

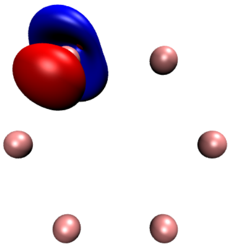

#MO 30

$\epsilon_i = 0.4827\ E_\mathrm{h}$
$\varepsilon_i = -0.0024\ E_\mathrm{h}$
$S_i = 0.0813$
$|-\rangle = 0.987$
$|\downarrow\rangle = 0.004$
$|\uparrow\rangle = 0.004$
$|\downarrow\uparrow\rangle = 0.004$

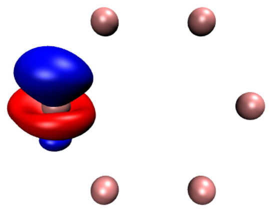

#MO 31

$\epsilon_i = 0.4872\ E_\mathrm{h}$
$\varepsilon_i = -0.0024\ E_\mathrm{h}$
$S_i = 0.0825$
$|-\rangle = 0.987$
$|\downarrow\rangle = 0.005$
$|\uparrow\rangle = 0.005$
$|\downarrow\uparrow\rangle = 0.004$

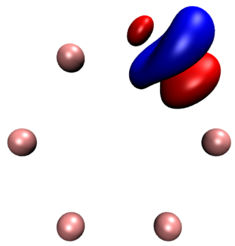

#MO 32

$\epsilon_i = 0.4872\ E_\mathrm{h}$
$\varepsilon_i = -0.0024\ E_\mathrm{h}$
$S_i = 0.0826$
$|-\rangle = 0.987$
$|\downarrow\rangle = 0.005$
$|\uparrow\rangle = 0.005$
$|\downarrow\uparrow\rangle = 0.004$

FIG. S16. $Be_6$ $R = 3.5$ Å: Foster-Boys localized active space molecular orbitals #25 to #32 with their corresponding diagonal Fock matrix element $\epsilon_i$, 1-orbital increment $\varepsilon_i$, 1-orbital entropy $S_i$ and orbital occupations $\omega_{i,\alpha} = \{|-\rangle, |\downarrow\rangle, |\uparrow\rangle, |\downarrow\uparrow\rangle\}$. Isosurfaces are plotted at $|\psi(\vec{r})| = 0.05\ a_0^{-1.5}$).

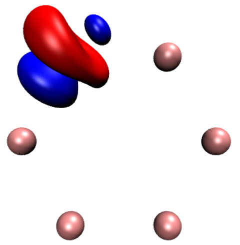

#MO 33

$\epsilon_i = 0.4872\ E_\mathrm{h}$
$\varepsilon_i = -0.0024\ E_\mathrm{h}$
$S_i = 0.0824$
$|-\rangle = 0.987$
$|\downarrow\rangle = 0.005$
$|\uparrow\rangle = 0.005$
$|\downarrow\uparrow\rangle = 0.004$

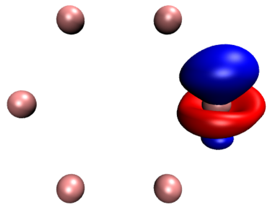

#MO 34

$\epsilon_i = 0.4872\ E_\mathrm{h}$
$\varepsilon_i = -0.0024\ E_\mathrm{h}$
$S_i = 0.0826$
$|-\rangle = 0.987$
$|\downarrow\rangle = 0.005$
$|\uparrow\rangle = 0.005$
$|\downarrow\uparrow\rangle = 0.004$

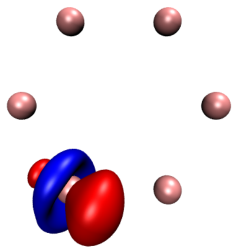

#MO 35

$\epsilon_i = 0.4873\ E_\mathrm{h}$
$\varepsilon_i = -0.0024\ E_\mathrm{h}$
$S_i = 0.0823$
$|-\rangle = 0.987$
$|\downarrow\rangle = 0.005$
$|\uparrow\rangle = 0.005$
$|\downarrow\uparrow\rangle = 0.004$

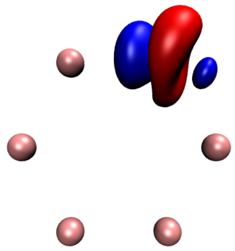

#MO 36

$\epsilon_i = 0.4873\ E_\mathrm{h}$
$\varepsilon_i = -0.0024\ E_\mathrm{h}$
$S_i = 0.0823$
$|-\rangle = 0.987$
$|\downarrow\rangle = 0.005$
$|\uparrow\rangle = 0.005$
$|\downarrow\uparrow\rangle = 0.004$

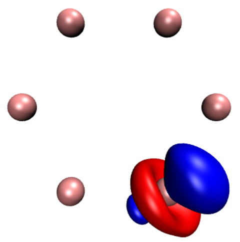

#MO 37

$\epsilon_i = 0.4873\ E_\mathrm{h}$
$\varepsilon_i = -0.0024\ E_\mathrm{h}$
$S_i = 0.0823$
$|-\rangle = 0.987$
$|\downarrow\rangle = 0.005$
$|\uparrow\rangle = 0.005$
$|\downarrow\uparrow\rangle = 0.004$

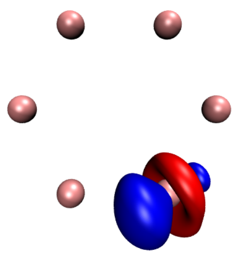

#MO 38

$\epsilon_i = 0.4873\ E_\mathrm{h}$
$\varepsilon_i = -0.0024\ E_\mathrm{h}$
$S_i = 0.0823$
$|-\rangle = 0.987$
$|\downarrow\rangle = 0.005$
$|\uparrow\rangle = 0.005$
$|\downarrow\uparrow\rangle = 0.004$

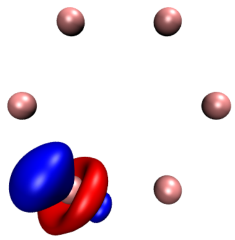

#MO 39

$\epsilon_i = 0.4873\ E_\mathrm{h}$
$\varepsilon_i = -0.0024\ E_\mathrm{h}$
$S_i = 0.0825$
$|-\rangle = 0.987$
$|\downarrow\rangle = 0.005$
$|\uparrow\rangle = 0.005$
$|\downarrow\uparrow\rangle = 0.004$

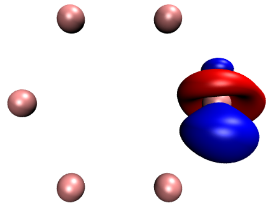

#MO 40

$\epsilon_i = 0.4873\ E_\mathrm{h}$
$\varepsilon_i = -0.0024\ E_\mathrm{h}$
$S_i = 0.0825$
$|-\rangle = 0.987$
$|\downarrow\rangle = 0.005$
$|\uparrow\rangle = 0.005$
$|\downarrow\uparrow\rangle = 0.004$

FIG. S17. $Be_6$ $R = 3.5$ Å: Foster-Boys localized active space molecular orbitals #33 to #40 with their corresponding diagonal Fock matrix element $\epsilon_i$, 1-orbital increment $\varepsilon_i$, 1-orbital entropy $S_i$ and orbital occupations $\omega_{i,\alpha} = \{|-\rangle, |\downarrow\rangle, |\uparrow\rangle, |\downarrow\uparrow\rangle\}$. Isosurfaces are plotted at $|\psi(\vec{r})| = 0.05\ a_0^{-1.5}$).

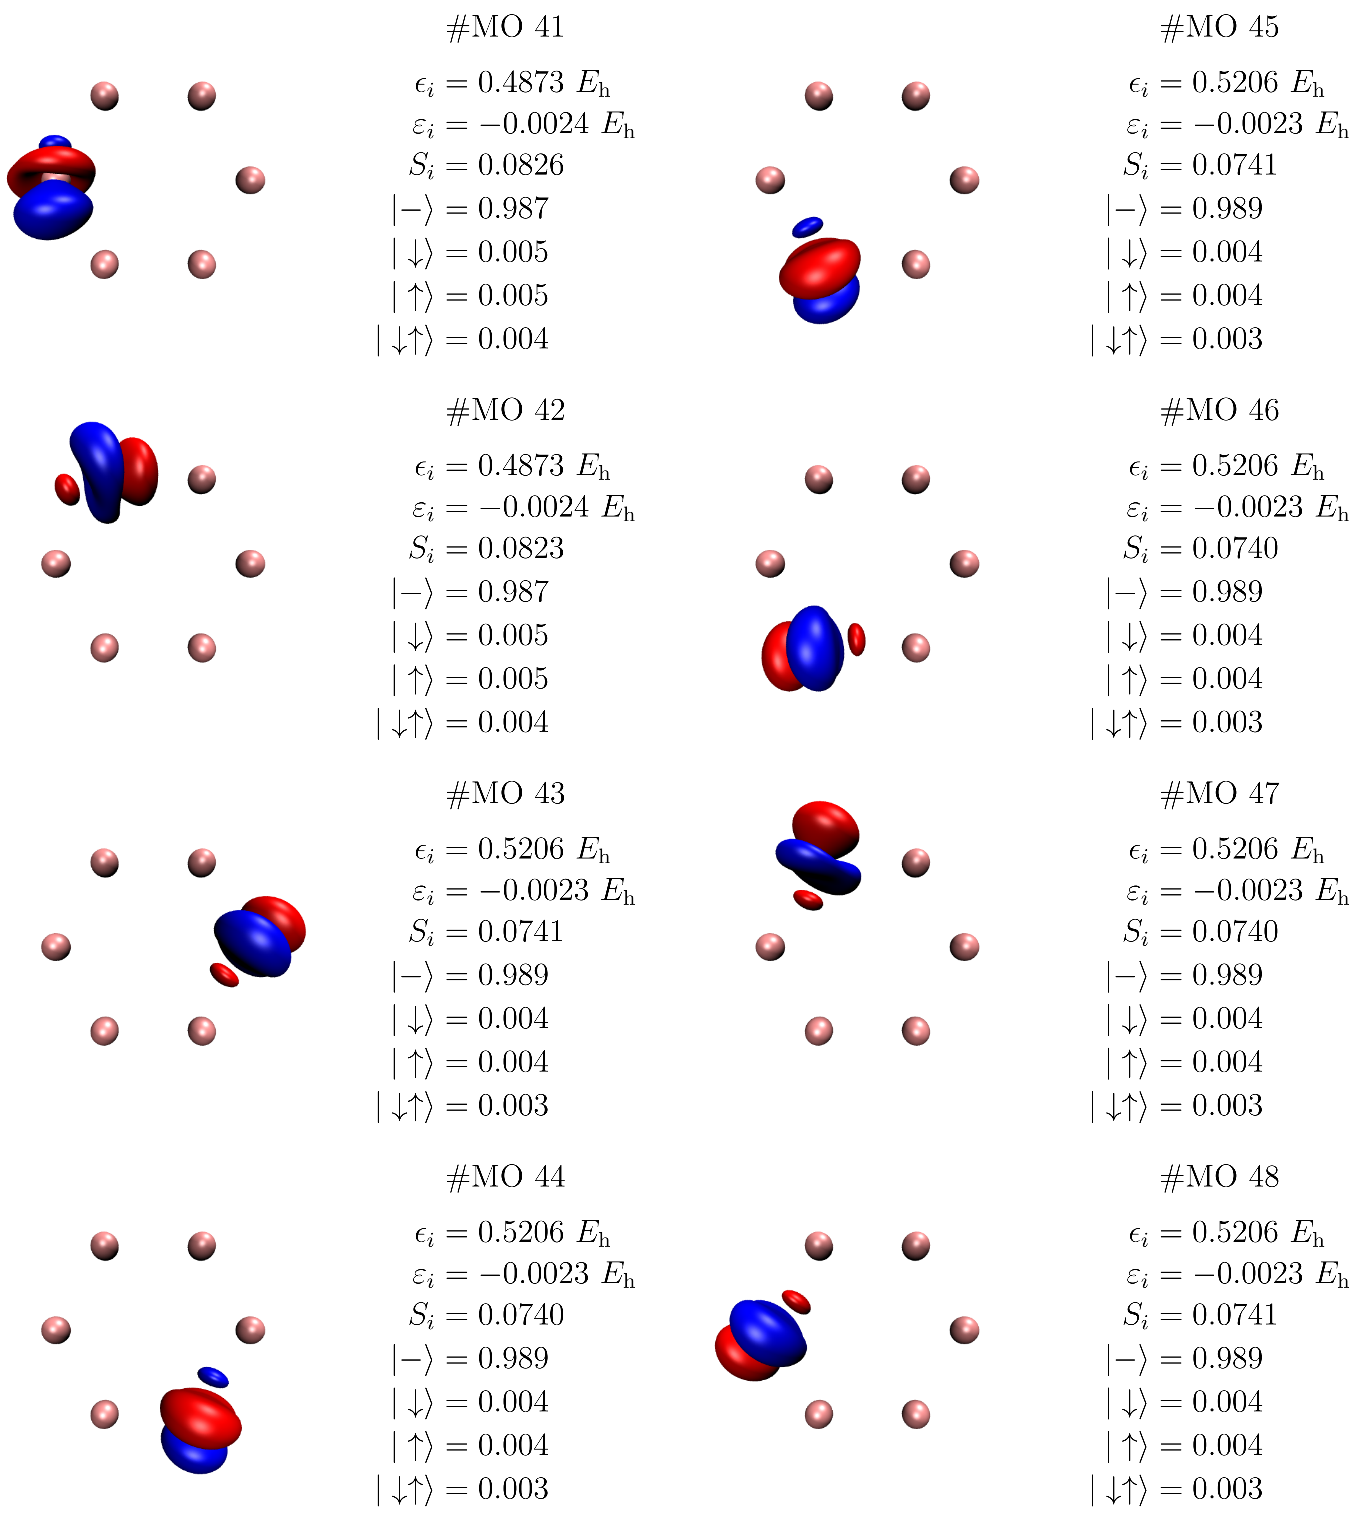


FIG. S18. $Be_6$ $R = 3.5$ Å: Foster-Boys localized active space molecular orbitals #41 to #48 with their corresponding diagonal Fock matrix element $\epsilon_i$, 1-orbital increment $\varepsilon_i$, 1-orbital entropy $S_i$ and orbital occupations $\omega_{i,\alpha} = \{|{-}\rangle, |{\downarrow}\rangle, |{\uparrow}\rangle, |{\downarrow\uparrow}\rangle\}$. Isosurfaces are plotted at $|\psi(\vec{r})| = 0.05\ a_0^{-1.5}$).

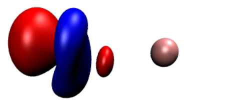

#MO 49

$\epsilon_i = 0.5206\ E_\mathrm{h}$
$\varepsilon_i = -0.0023\ E_\mathrm{h}$
$S_i = 0.0740$
$|-\rangle = 0.989$
$|\downarrow\rangle = 0.004$
$|\uparrow\rangle = 0.004$
$|\downarrow\uparrow\rangle = 0.003$

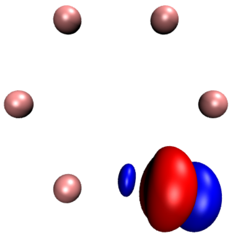

#MO 50

$\epsilon_i = 0.5206\ E_\mathrm{h}$
$\varepsilon_i = -0.0023\ E_\mathrm{h}$
$S_i = 0.0740$
$|-\rangle = 0.989$
$|\downarrow\rangle = 0.004$
$|\uparrow\rangle = 0.004$
$|\downarrow\uparrow\rangle = 0.003$

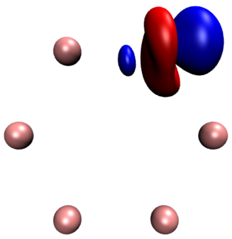

#MO 51

$\epsilon_i = 0.5206\ E_\mathrm{h}$
$\varepsilon_i = -0.0023\ E_\mathrm{h}$
$S_i = 0.0740$
$|-\rangle = 0.989$
$|\downarrow\rangle = 0.004$
$|\uparrow\rangle = 0.004$
$|\downarrow\uparrow\rangle = 0.003$

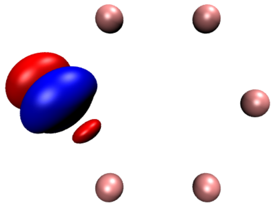

#MO 52

$\epsilon_i = 0.5206\ E_\mathrm{h}$
$\varepsilon_i = -0.0023\ E_\mathrm{h}$
$S_i = 0.0742$
$|-\rangle = 0.989$
$|\downarrow\rangle = 0.004$
$|\uparrow\rangle = 0.004$
$|\downarrow\uparrow\rangle = 0.003$

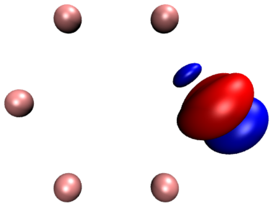

#MO 53

$\epsilon_i = 0.5206\ E_\mathrm{h}$
$\varepsilon_i = -0.0023\ E_\mathrm{h}$
$S_i = 0.0741$
$|-\rangle = 0.989$
$|\downarrow\rangle = 0.004$
$|\uparrow\rangle = 0.004$
$|\downarrow\uparrow\rangle = 0.003$

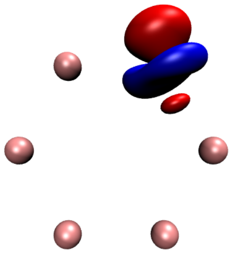

#MO 54

$\epsilon_i = 0.5206\ E_\mathrm{h}$
$\varepsilon_i = -0.0023\ E_\mathrm{h}$
$S_i = 0.0741$
$|-\rangle = 0.989$
$|\downarrow\rangle = 0.004$
$|\uparrow\rangle = 0.004$
$|\downarrow\uparrow\rangle = 0.003$

FIG. S19. $Be_6$ $R = 3.5$ Å: Foster-Boys localized active space molecular orbitals #49 to #54 with their corresponding diagonal Fock matrix element $\epsilon_i$, 1-orbital increment $\varepsilon_i$, 1-orbital entropy $S_i$ and orbital occupations $\omega_{i,\alpha} = \{|-\rangle, |\downarrow\rangle, |\uparrow\rangle, |\downarrow\uparrow\rangle\}$. Isosurfaces are plotted at $|\psi(\vec{r})| = 0.05\ a_0^{-1.5}$).
